# Supplementary material for: AquaMILR: Mechanical intelligence simplifies control of undulatory robots in cluttered fluid environments
Source: arXiv:2407.01733 source file (2024-09-27)
Supplement: Supplementary file 1 [file SI_movie.tex]

https://www.dropbox.com/scl/fi/r3vwtc5vgykojtg0ml298/si_movie.mp4?rlkey=bywlmmesxnqonrcworm1qxtue&dl=0
